# Supplementary material for: Attentional Local Contrast Networks for Infrared Small Target Detection
Source: arXiv:2012.08573 source file (2020-12-15)
Supplement: Supplementary file 1 [file appendix.tex]

% !TEX root = ../main.tex
%\bibliography{../reference}
